# Supplementary material for: Shadow Ansatz for the Many-Fermion Wave Function in Scalable Molecular Simulations on Quantum Computing Devices
Source: arXiv:2408.11026 source file (2024-08-20)
Supplement: Supplementary file 1 [file SI.pdf]

# Supplemental Material: Shadow Ansatz for the Many-Fermion Wave Function in Scalable Molecular Simulations on Quantum Computing Devices

Yuchen Wang, Irma Avdic and David A. Mazziotti[1, *]

[1] *Department of Chemistry and The James Franck Institute, The University of Chicago, Chicago, Illinois 60637, USA*

(Dated: Submitted August 8, 2024)

## I. CALIBRATION DATA FOR IBM CLEVELAND

This work utilized a 127-qubit IBM Quantum device ibm_cleveland, which is one of the IBM Eagle Processors [1]. The calibration details are given in Table I.

TABLE I. Calibration data for selected qubits in IBM Cleveland (last accessed on 07/22/2024). RO for read-out assignment error. For ECR error, the number in parentheses is connecting qubit.

| Qubit No. | $T_1$ ($\mu s$) | $T_2$ ($\mu s$) | RO ($10^{-2}$) | ECR error ($10^{-3}$) | gate time(ns) | freq. (GHz) |
|---|---|---|---|---|---|---|
| 44 | 235.22 | 249.70 | 1.46 | | | 4.814 |
| 45 | 220.08 | 363.08 | 1.37 | 9.841(44) | 590.222 | 4.612 |
| 46 | 299.29 | 327.65 | 2.13 | 4.160(45) | 590.222 | 4.829 |

## II. QUBIT TAPERING IN $H_3$ SIMULATION

The qubit tapering technique in this work follows the work by Bravyi et. al. [2] The implementation is also documented in appendix B3 of ref. [3]. After mapping the Hamiltonian to qubits, we aim to find a set of Pauli strings that commute with this qubit Hamiltonian. These Pauli strings can be viewed as symmetry conditions due to either the conserving of $N$ and $S_z$ numbers for chemistry problems or point group symmetry for particular molecular geometries [4].

The procedure to find these Pauli strings in this work is presented here. We mapped the fermionic Hamiltonian to qubits via Jordan-Wigner mapping [5, 6]. The qubit Hamiltonian is put in a checksum representation to construct the parity check matrix. By performing Gaussian elimination on the parity check matrix, we can find the null space, of which the elements correspond to symmetries of the Hamiltonian, and the rank of the null space equals the number of qubits that we can taper. Specifically, the symmetries we find for linear $H_3$ are

$$S = \{Z_1Z_2Z_3, Z_2Z_5, Z_2Z_4Z_5\}, \tag{1}$$

which allows us to taper off three qubits from a six-qubit Jordan-Wigner Hamiltonian.

## III. ADDITIONAL IMPLEMENTATION DETAILS

We use Qiskit 1.0 to interface with quantum hardware [7]. Certain techniques are used to reduce the circuit depth on current NISQ devices. We apply a threshold with two conditions, first, the coefficients of certain Pauli terms should be greater than 0.01, and second, provided that multiple terms satisfy the condition, they are attached to the circuits in a sequence based on their coefficients. The new unitaries are only appended to the current wave function when the energies decrease after applying the unitaries, which is not always the case when the circuits become deep. For every run, the circuits are optimized with a transpiler in Qiskit at optimization level 3. We use the resilience

* damazz@uchicago.edu

level 2 with default settings for Qiskit runtime error mitigation, which contains certain measurement twirling, gate twirling, and zero noise extrapolation techniques. For every calculation, we apply 4096 shots per experiment and the experiments are repeated 10 times to obtain the mean and standard deviation in Fig. 4.


[1] IBM-Quantum, https://quantum-computing.ibm.com/ (2024).

[2] S. Bravyi, J. M. Gambetta, A. Mezzacapo, and K. Temme, Tapering off qubits to simulate fermionic hamiltonians, arXiv preprint arXiv:1701.08213 10.48550/arXiv.1701.08213 (2017).

[3] S. E. Smart, J.-N. Boyn, and D. A. Mazziotti, Resolving correlated states of benzyne with an error-mitigated contracted quantum eigensolver, Phys. Rev. A **105**, 022405 (2022).

[4] K. Setia, R. Chen, J. E. Rice, A. Mezzacapo, M. Pistoia, and J. D. Whitfield, Reducing qubit requirements for quantum simulations using molecular point group symmetries, J. Chem. Theory Comput. **16**, 6091 (2020).

[5] P. Jordan and E. Wigner, Über das paulische Äquivalenzverbot, Z. Physik **47**, 631–651 (1928).

[6] E. Fradkin, Jordan-wigner transformation for quantum-spin systems in two dimensions and fractional statistics, Phys. Rev. Lett. **63**, 322–325 (1989).

[7] Qiskit contributors, Qiskit: An open-source framework for quantum computing (2024).
